# Supplementary material for: Adaptive Cross-Packet HARQ
Source: arXiv:1606.05182 source file (2016-06-16)
Supplement: Supplementary file 1 [file Appendix_Decoding_Proof.tex]

%!TEX root =  ../HARQ.joint.codec.tex
\section{Decoding conditions of \gls{xp}}\label{Sec:Decoding_Proof}

In this appendix, we outline the proof of the decoding conditions \eqref{dec.1} and \eqref{dec.2}, stated in the following  \lemref{lemma:DecodingConditions}. We consider an HARQ-code $c \in\mathcal{C}$

Given a sequence length $n\in\mathbb{N}$, an HARQ-code $c \in\mathcal{C}(n,R_1,R_2)$ is a tuple of functions $(C_1,C_2,C_3,C_4)$ defined by

{
\begin{footnotesize}
\begin{eqnarray}
&C_1& : \mathcal{M}_1  \longrightarrow \mathcal{X}_1^n,\label{eq:Code1}\\
&C_2& :  \mathcal{K}_1 \times \mathcal{Y}_1^n  \longrightarrow \{\ack_1,\nack_1 \} \times \mathcal{M}_1, \label{eq:Code2}\\
&C_3&: \mathcal{M}_1\times \mathcal{M}_2 \times \{\ack_1,\nack_1 \} \longrightarrow \mathcal{X}_2^{ n},\label{eq:Code3}\\
&C_4& : \mathcal{Y}_1^n \times \mathcal{Y}_2^n \times  \mathcal{K}_1 \times \mathcal{K}_2 \rightarrow \{\ack_2,\nack_2 \} \times \mathcal{M}_1\times \mathcal{M}_2 .\label{eq:Code4}
\end{eqnarray}
\end{footnotesize}
}
where, for notation convenience, $\mathcal{X}_k^n, \mathcal{Y}_k^n, \mathcal{M}_k, \mathcal{K}_k$ denote the set of input symbols sequence, the set of possible outputs, the set of messages $\mfm_{k}$ and the set of  channel states in the $k$th round, respectively. In our case, the channel state is totally  characterized by $\SNR_{k}$, thus, $\mathcal{K}_k=\Real_{+}~\forall k$. However, we will use $\mathcal{K}_k$ to keep the generality of the decoding conditions.  

%The set of HARQ-code $\mathcal{C}(n,R_1,R_2)$ is defined by \eqref{eq:Code1}-\eqref{eq:Code4}.

\begin{lemma}[Decoding conditions]\label{lemma:DecodingConditions}
For all $\varepsilon>0$, there exists a  $\bar{n}\in \mathbb{N}$ such that for all $n\geq \bar{n}$, there exists a HARQ-code $c^{\star} \in\mathcal{C}(n,R_1,R_2)$ such that for all channel states $k_{1} \in \mathcal{K}_1$ and $k_{2} \in \mathcal{K}_2$ satisfying,
\begin{eqnarray}
R_1 &\leq& \mfI(X_1 ; Y_1 |k_{1}) - 4 \varepsilon , \label{eq:Rate1} \\
R_1 +  R_2 &\leq& \mfI(X_1 ; Y_1 |k_{1}) + \mfI(X_2 ; Y_2 |k_{2}) - 4 \varepsilon, \label{eq:Rate2} 
\end{eqnarray}
the error probability is bounded below $\varepsilon$, \ie
%\begin{footnotesize}
\begin{eqnarray}
\mathcal{P}\bigg( \Big\{ \mfm_1\neq \hat{\mfm_1} \Big\} \cup \Big \{   \mfm_2\neq \hat{\mfm_2} \Big\}  \bigg|\;c^{\star},  k_{1}, k_{2}  \;\bigg) \leq \varepsilon.\label{eq:DefErrorProbaLz}
\end{eqnarray}
%\end{footnotesize}
\end{lemma}

\begin{proof}[Proof of Lemma \ref{lemma:DecodingConditions}]
We consider a random HARQ-code $c \in \mathcal{C}(n,R_1,R_2)$, defined as follows:
\begin{itemize}
\item[$\bullet$] \textit{Random codebook:} we generate $|\mathcal{M}_1|= 2^{n \cdot R_1 } $ sequences $x_1^n$ and $|\mathcal{M}_1 \times \mathcal{M}_2|= 2^{n \cdot ( R_1 + R_2 )} $ sequences $x_2^n$, drawn from the i.i.d.  distribution $\mathcal{P}^{\star}(x)$. The index $n$ is added to emphasize the length of sequence $n$. In our context, $n=\Ns$.
\item[$\bullet$] \textit{Encoding function:} as explained in \secref{Sec:joint.codec}, the encoder starts by sending $x_1^n$ which corresponds to the message $\mfm_1 \in \mathcal{M}_1$. If the encoder receives a $\nack_1$ message, it sends $x_2^n$ corresponding to the pair of messages $[\mfm_1 , \mfm_2]  \in \mathcal{M}_1 \times \mathcal{M}_2$. Otherwise a new transmission process starts. 
\item[$\bullet$] \textit{Decoding function:}  if the channel states $( k_{1}, k_{2})$ satisfy equations \eqref{eq:Rate1} and \eqref{eq:Rate2}, then the decoder finds a pair of messages $[\mfm_1,\mfm_2]$
 such that the following sequences of symbols are jointly typical:
\begin{eqnarray}
\Big(x_1^n , y_1^n  \Big) &\in& A_{\varepsilon}^{{\star}{n}}\big(\mathcal{Q}(x,y|k_{1})\big), \label{eq:JointTypical1}\\
\Big(x_2^n , y_2^n  \Big) &\in& A_{\varepsilon}^{{\star}{n}}\big(\mathcal{Q}(x,y|k_{2})\big) \label{eq:JointTypical2}.
\end{eqnarray}
For each transmission $l \in \{1,2\}$, the joint probability distribution $\mathcal{Q}(x,y|s_{l}) = \mathcal{P}^{\star}(x) \cdot T(y|x,s_{l})$ is defined with respect to the channel state $k_{l}\in\mathcal{K}_l$. The decoder returns the messages $(m_1,m_2) $. What are $A_{\varepsilon}^{{\star}{n}}\big(\mathcal{Q}(x,y|k_{1})\big), \mathcal{P}^{\star}(x) \text{and} T(y|x,s_{l})$?
\item[$\bullet$] \textit{Error} is declared when sequences  are not jointly typical. 
\end{itemize}

\begin{figure}[!ht]
\begin{center}
%\begin{tiny}
%\begin{large}
\psset{xunit=0.7cm,yunit=0.5cm}
\begin{pspicture}(-5.3,10.4)(9,17.3)
\psellipse(2,16)(3,0.7)
\psellipse(2,14)(3,0.7)
\psdots(2,12.8)(2,12.5)(2,12.2)
\psellipse(2,11)(3,0.7)
\psdots(2,16)
\rput[u](4,17.3){$x_2\sim  \mathcal{P}_{\sf{x}}^{\star \times n } $}
\psline[linewidth=1pt]{-}(-2,16)(2,16)
\psline[linewidth=1pt]{-}(2,15)(2,16)
\rput[u](-2.4,16){$m_1$}
\rput[u](2.4,15){$m_2$}
\rput[u](-3.5,13.5){$|\mathcal{M}_1  |= 2^{n R_1  } $}
\psbrace[linecolor=black,ref=rC](-1,17)(-1,10){}
\rput[u](-2.5,17.3){$|\mathcal{M}_1 \times \mathcal{M}_2 | = 2^{n \cdot (R_1 + R_2) } $}
\rput[u](6,15){$|\mathcal{M}_2  |= 2^{n R_2  } $}
\end{pspicture}
%\end{tiny}
%\end{large}
\caption{Random generation of the codebook: $x_2$. }
%for HARQ-code ${c}  \in\mathcal{C}(n,R_1,R_2)$.}
\end{center}
\label{figure:BinningLeszekCode}
\end{figure}

\textbf{Error events.} We define the following error events:  
\begin{scriptsize}
\begin{itemize}
\item[$\bullet$]$E_0=\bigg\{(x_1^n, y_1^n)\notin A_{\varepsilon}^{{\star}{n}}\big(\mathcal{Q}(x,y|k_{1})\big) \bigg\}$\\ \qquad\qquad $  \qquad \cup \bigg\{(x_2^n, y_2^n)\notin A_{\varepsilon}^{{\star}{n}}\big(\mathcal{Q}(x,y|k_{2})\big) \bigg\}$.\\
\item[$\bullet$]$E_1 =\bigg\{\exists m'_1 \neq m_1,\text{ s.t. } \big( x_1^n(m'_1) , y_1^n\big) \in  A_{\varepsilon}^{{\star}{n}}\big(Q(x,y|k_{1})\big)\bigg\}$.\\
\item[$\bullet$]$E_{2} =\bigg\{\exists (m'_1,m'_2) \neq (m_1,m_2),\text{ s.t. }\Big\{ \big( x_1^n(m'_1) , y^n_1\big) \in  A_{\varepsilon}^{{\star}{n}}\big(Q(x,y|k_{1})\big) \Big\} \cap \Big\{  \big( x_2^n(m'_1,m'_2) , y_2^n\big) \in  A_{\varepsilon}^{{\star}{n}}\big(Q(x,y|k_{2})\big) \Big\} \bigg\}$.\\
\item[$\bullet$]$E_{3} =\bigg\{\exists m'_1\neq m_1,\text{ s.t. }\Big\{ \big( x_1^n(m'_1) , y^n_1\big) \in  A_{\varepsilon}^{{\star}{n}}\big(Q(x,y|k_{1})\big) \Big\} \cap \Big\{  \big( x_2^n(m'_1,m_2) , y_2^n\big) \in  A_{\varepsilon}^{{\star}{n}}\big(Q(x,y|k_{2})\big) \Big\} \bigg\}$.\\
\item[$\bullet$]$E_{4} =\bigg\{\exists m'_2 \neq m_2,\text{ s.t. } \big( x_2^n(m_1,m'_2) , y_2^n\big) \in  A_{\varepsilon}^{{\star}{n}}\big(Q(x,y|k_{2})\big)\bigg\}$.\\
\end{itemize}
\end{scriptsize}

\textbf{Upper bound on an error event $E_{2}$.} We consider the error event $E_{2} $ and we  provide an upper bound on the expected probability, that is valid for all  channel states $(k_{1}  , k_{2})$ that satisfy equations \eqref{eq:Rate1} and \eqref{eq:Rate2}.

\begin{tiny}
\begin{eqnarray}
&&  \mathbb{E}_c\bigg[\mathcal{P}\bigg(\exists (m'_1,m'_2) \neq (m_1,m_2),\text{ s.t. }\Big\{ \big( X_1^n(m'_1) , Y^n_1\big) \in  A_{\varepsilon}^{{\star}{n}}\big(Q(x,y|k_{1})\big) \Big\} \nonumber\\ 
&&\cap \Big\{  \big( X_2^n(m'_1,m'_2) , Y_2^n\big) \in  A_{\varepsilon}^{{\star}{n}}\big(Q(x,y|k_{2})\big) \Big\}   \bigg)\bigg] \nonumber  \\ 
&\leq&  \sum_{(m'_1,m'_2) \atop \neq (m_1,m_2)} 
\sum_{ (x_1^n, y_1^n) \in \atop  A_{\varepsilon}^{\star n}(\mathcal{Q}(x,y|k_{1}))} 
 \mathbb{E}_c\bigg[\mathcal{P}\bigg(  \big( X_1^n(m'_1) , Y^n_1\big) = (x_1^n, y_1^n)  \bigg)\bigg]  \nonumber\\ 
&& \times \sum_{ (x_2^n, y_2^n) \in \atop  A_{\varepsilon}^{\star n}(\mathcal{Q}(x,y|k_{2})} 
\mathbb{E}_c\bigg[\mathcal{P}\bigg(    \big( X_2^n(m'_1,m'_2) , Y_2^n\big)  =   (x_2^n, y_2^n)  \bigg)\bigg] \label{eq:ErrorSecond2}  \\
&\leq&  \sum_{(m'_1,m'_2) \atop \neq (m_1,m_2)} 
\sum_{ (x_1^n, y_1^n) \in \atop  A_{\varepsilon}^{\star n}(\mathcal{Q}(x,y|k_{1}))} 
 \mathbb{E}_c\bigg[\mathcal{P}\bigg( X_1^n(m'_1) = x_1^n  \bigg)\bigg]   \times  \mathbb{E}_c\bigg[\mathcal{P}\bigg( Y^n_1 = y_1^n  \bigg)\bigg]   \nonumber\\ 
&& \times \sum_{ (x_2^n, y_2^n) \in \atop  A_{\varepsilon}^{\star n}(\mathcal{Q}(x,y|k_{2}))} 
\mathbb{E}_c\bigg[\mathcal{P}\bigg(    X_2^n(m'_1,m'_2)  = x_2^n  \bigg)\bigg]   \times  \mathbb{E}_c\bigg[\mathcal{P}\bigg(   Y_2^n  =    y_2^n  \bigg)\bigg] \label{eq:ErrorSecond4}  \\
&\leq& 2^{n \cdot \bigg(\textsf{R}_1 + \textsf{R}_2  - \mfI(X_1;Y_1|k_{1})  - \mfI(X_2;Y_2|k_{2})   + 3\varepsilon  \bigg)}   \label{eq:ErrorSecond5}  \\
&\leq&  2^{ -  n \cdot \varepsilon }.\label{eq:ErrorSecond8}
\end{eqnarray}
\end{tiny}
Equation \eqref{eq:ErrorSecond2} comes from Boole's inequality and from the independence of  sequences $ \big( X_1^n(m'_1) , Y^n_1\big)$ of the first block with respect to $\big( X_2^n(m'_1,m'_2) , Y_2^n\big)$ of the second block.\\
Equation \eqref{eq:ErrorSecond4} comes from the independence of the codewords $X _1^n(m'_1)$ with $(X _1^n(m_1), Y _1^n)$ and $X_2^n(m'_1,m'_2)$ with $(x_2, Y _2^n)$. \\
Equation \eqref{eq:ErrorSecond5} comes from the properties of the typical sequences, stated pp. 26 in  \cite{ElGammal11_Book} and the cardinality of the sets $\mathcal{M}_1$ and $\mathcal{M}_2$, in the random codebook.\\
Equation \eqref{eq:ErrorSecond8}  comes from the equation \eqref{eq:Rate2}, that is satisfied for the channel states $(k_{1}  , k_{2})$.

There exists a $n_2\in \mathbb{N}$ such that for all $n\geq n_2$, the expected probability of event $E_{2}$ is bounded for all channel states $(k_{1}  , k_{2})$.
\begin{eqnarray}
\mathbb{E}_c\bigg[\mathcal{P}\bigg(E_{2} \bigg|\;c,  k_{1}, k_{2} \bigg)\bigg] \leq \varepsilon.\label{eq:ErrorSecond6}
\end{eqnarray}
This proof relies on the jointly typical lemma, stated in \cite{ElGammal11_Book} page 29, and the same arguments provide upper bounds for the error events $E_{3}$ and $E_{4}$. This proves the existence of an HARQ-code $c^{\star} \in \mathcal{C}(n,R_1,R_2)$ with  error probability bounded by $\varepsilon>0$ for all channel states $( k_{1}, k_{2} )$ satisfying \eqref{eq:Rate1}-\eqref{eq:Rate2}:
\begin{eqnarray}
\mathcal{P}\bigg( \Big\{ M_1\neq \hat{M_1} \Big\} \cup \Big \{   M_2\neq \hat{M_2} \Big\}  \bigg|\;c^{\star},  k_{1}, k_{2}  \;\bigg) \leq \varepsilon.\label{eq:DefErrorProbaLz}
\end{eqnarray}
This concludes the proof of Lemma \ref{lemma:DecodingConditions}.

\end{proof}
