# Supplementary material for: Adaptive Cross-Packet HARQ
Source: arXiv:1606.05182 source file (2016-06-16)
Supplement: Supplementary file 2 [file Appendix_Optimal_policy_K2.tex]

%!TEX root =  ../HARQ.joint.codec.tex
%%%%%%
\section{Analytical solution of the optimization problem \eqref{op.throughput.definition.RR}}\label{Sec:OptimalAdaptation.Analytic}

In this appendix, we will solve analytically the optimization problem \eqref{op.throughput.definition.RR} when $\kmax=2$ and the rate of the first transmission is constant and equals to $\R_{1}$. That is, the objectif is to solve the following optimization problem:

\begin{align}\label{op.throughput.definition.RR.2} 
&\displaystyle{\eta^\xp_2=\max_{ \R_{2}(I_{1})} \frac{\Ex_{\{I_{1},I_{2}\}}\Big[\R_{1}\IND{I_{1}\ge \R_{1}}\Big]}{1+f_{1}}+}\nonumber \\ 
&\displaystyle{\frac{\Ex_{\{I_{1},I_{2}\}}\Big[(\R_{1}+ \R_{2}(I_{1}))\IND{I_{1}\le \R_{1} \wedge I_{1}+I_{2}\ge \R_{1}+\R_{2}(I_{1})}\Big]}{1+f_{1}}}\\
&\displaystyle{=\max_{ \R_{2}(I_{1})} \frac{\R_{1}(1-f_{1})}{1+f_{1}}}+\nonumber \\ 
&\displaystyle{\frac{\Ex_{\{I_{1},I_{2}\}}\Big[(\R_{1}+ \R_{2}(I_{1}))\IND{I_{1}\le \R_{1} \wedge I_{1}+I_{2}\ge \R_{1}+\R_{2}(I_{1})}\Big]}{1+f_{1}}},
\end{align}
where $f_{1}=\Pr\{I_{1}<\R_{1}\}$ is independent of $\R_{2}(\cd)$. Thus, \eqref{op.throughput.definition.RR.2} is equivalent to
\begin{align}\label{} 
\max_{ \R_{2}(I_{1})}& \Ex_{\{I_{1},I_{2}\}}\Big[(\R_{1}+ \R_{2}(I_{1})) \times \nonumber \\
& \IND{ I_{1}\le \R_{1} \wedge I_{1}+I_{2}\ge \R_{1}+\R_{2}(I_{1})}\Big].
\end{align}

Therefore, for each value of $I_{1}<\R_{1}$, the optimal $\R_{2}(I_{1})$ is given by
\begin{align}\label{} 
\R_{2}(I_{1})=\argmax_{R}~(\R_{1}+ R) \cd \cdf_{I_{2}}^{\tr{c}}(\R_{1}+R-I_{1}).
\end{align}
which is a simple one-dimension optimization problem. 

 For the particular case of Gaussian modulation when the \gls{mi} is given by $I_{k}=\log_{2}(1+\SNR_{k})$, it is easy to show that the optimal rate adaptation policy is given by the following closed-form
\begin{align}\label{eq:optimal.analitical.policy} 
\R_{2}(I_{1})=\max\big(0,\frac{W(2^{I_{1}} \SNRav )}{\log(2)}-R_{1}\big),
\end{align}
 where $W(.)$ is Lambert $W$ function defined as the solution of $x=W(x)\e^{W(x)}$. Thus, the optimal throughput is given by:
\begin{align}
&\eta^\xp_2=\frac{\R_{1}(1-f_{1})}{1+f_{1}}+\nonumber \\
& \frac{\Ex_{\{I_{1}\}}\Big[(\R_{1}+ \R_{2}(I_{1})) \cdf_{I_2}^{\tr{c}}(\R_{1}+\R_{2}(I_{1})-I_{1}) | I_1<\R_1\Big]}{1+f_{1}},
\end{align}
